# Supplementary material for: UCoDe: Unified Community Detection with Graph Convolutional Networks
Source: arXiv:2112.14822 source file (2023-11-02)
Supplement: Supplementary file 1 [file 99.supplementary.tex]

%!TEX root=../main.tex

\section{Supplementary material}


\input{tables/tbl-nmi-nonoverlapping}
\input{tables/tbl-f1-nonoverlapping}

Here we introduce some supplementary material for reproducing the experiments and provide additional analyses that are not part of the paper.

\subsection{Implementation and Experimental setup}
We release the implementation of \ourmethod at \url{https://anonymous.4open.science/r/UCODE-8DC7/}. 
Our code is compatible with python v3.8 or above. We implement \ourmethod using pytorch version 1.10.0. 

We evaluate our methods on a 14-core Intel Core i9 10940X 3.3GHz machine with 256GB RAM running python v3.8. 

\subsection{Data release}
The data used in our experiments is publicly available in the corresponding publications described in Section~\ref{sec:experiments}. We additionally release the data in our anonymous repository above. For all the experiments we use the original data, with no alteration or preprocessing.  


\subsection{Hyperparameter Experiments}
For transparency on the hyperparameter selection process, we share some experimental results in Figure~\ref{fig:supplementary} with regards to the hidden layer size and overlapping threshold parameter. The threshold was applied to the output of $\cmat^\top\bmat\cmat$ before the sigmoid with the logarithm as described in section \ref{solution:log}. As we can see, the results show that, while NMI in Figure~\ref{fig:tuning} increases with the dimensionality, modularity decreases. This confirms our hypothesis that modularity optimization alone does not suffice for community detection. 

\input{figs/supplementary_figs}

\subsection{Data for Figure~\ref{fig:nmi-nonoverlapping} and Figure~\ref{fig:f1-nonoverlapping}}

We report in Table~\ref{tbl:nmi-nonoverlapping} the raw data that generated the NMI results for non-overlapping communities in Figure~\ref{fig:nmi-nonoverlapping}. Similarly, Table~\ref{tbl:f1-nonoverlapping} reports the raw data for F1-score presented in Figure~\ref{fig:f1-nonoverlapping}. The figures reported in the paper are more easily readable and therefore we opted for such more intuitive presentation. 
